# Supplementary material for: Field theoretical approach to gravitational waves
Source: arXiv:1701.07794 ancillary file (2017-05-16)
Supplement: Supplementary file 1 [file Exercises.pdf]

# EXERCISES

These exercises were suggested during the lectures delivered by Professor van Holten at the 21st “*Saalburg*” Summer School. They constitute a supplement to the notes “Field theoretical approach to gravitational waves”.

## 1 Representation of the Poincaré group

### 1.1 Commutation relations for spin operators

Let  $(\Sigma_{\mu\nu})_\alpha^\beta$  be the representation of the spin operator on rank-1 fields

$$(\Sigma_{\mu\nu})_\alpha^\beta = \eta_{\mu\alpha}\delta_\nu^\beta - \eta_{\nu\alpha}\delta_\mu^\beta, \quad (1.1)$$

and let  $(\Sigma_{\mu\nu})_{\alpha\beta}^{\gamma\delta}$  be the representation of the spin operator on rank-2 fields

$$(\Sigma_{\mu\nu})_{\alpha\beta}^{\gamma\delta} = (\eta_{\mu\alpha}\delta_\nu^\gamma - \eta_{\nu\alpha}\delta_\mu^\gamma)\delta_\beta^\delta + \delta_\alpha^\gamma(\eta_{\mu\beta}\delta_\nu^\delta - \eta_{\nu\beta}\delta_\mu^\delta). \quad (1.2)$$

Show that, in both cases, the commutation relation is given by

$$[\Sigma_{\mu\nu}, \Sigma_{\kappa\lambda}] = \eta_{\nu\kappa}\Sigma_{\mu\lambda} - \eta_{\nu\lambda}\Sigma_{\mu\kappa} - \eta_{\mu\kappa}\Sigma_{\nu\lambda} + \eta_{\mu\lambda}\Sigma_{\nu\kappa}. \quad (1.3)$$

### 1.2 Eigenvalues of the Casimir operators

Let us define the two Casimir invariants

$$Z^2 = P^\mu \Sigma_{\mu\lambda} P^\nu \Sigma_\nu^\lambda, \quad W^2 = \frac{1}{2} P^2 \Sigma^2 - Z^2. \quad (1.4)$$

a) Show that for a vector field  $A_\alpha$ , one has

$$(Z^2 A)_\alpha = -P^2 A_\alpha - 2P_\alpha P^\beta A_\beta, \quad (1.5)$$

$$(W^2 A)_\alpha = -2P^2 A_\alpha + 2P_\alpha P^\beta A_\beta. \quad (1.6)$$

b) Show that the eigenvalue equations

$$P^2 A_\alpha = m^2 A_\alpha, \quad (Z^2 A)_\alpha = \lambda A_\alpha, \quad (W^2 A)_\alpha = \kappa A_\alpha, \quad (1.7)$$

have 2 solutions:

(i) a longitudinal scalar solution

$$\lambda = -3m^2, \quad \kappa = 0, \quad A_\alpha = P_\alpha \Phi, \quad P^2 \Phi = m^2 \Phi; \quad (1.8)$$

(ii) a transverse vector solution

$$\lambda = -m^2, \quad \kappa = -2m^2, \quad P^2 A_\alpha = m^2 A_\alpha, \quad P^\alpha A_\alpha = 0. \quad (1.9)$$

c) Show that for a symmetric tensor field  $A_{\alpha\beta}$ , one has

$$\begin{aligned} (Z^2 A)_{\alpha\beta} = & -2P^2 A_{\alpha\beta} - 4P_\alpha P^\gamma A_{\beta\gamma} - 4P_\beta P^\gamma A_{\alpha\gamma} + 2\eta_{\alpha\beta} P^\gamma P^\delta A_{\gamma\delta} \\ & + 2P_\alpha P_\beta A_\gamma{}^\gamma, \end{aligned} \quad (1.10)$$

$$\begin{aligned} (W^2 A)_{\alpha\beta} = & -6P^2 A_{\alpha\beta} + 4P_\alpha P^\gamma A_{\beta\gamma} + 4P_\beta P^\gamma A_{\alpha\gamma} - 2P_\alpha P_\beta A_\gamma{}^\gamma \\ & + 2\eta_{\alpha\beta} (P^2 A_\gamma{}^\gamma - P^\gamma P^\delta A_{\gamma\delta}). \end{aligned} \quad (1.11)$$

d) Show that the eigenvalue equations, appropriately generalised from those of Eqs (1.7), have 4 solutions:

(i) a trace-like scalar

$$\lambda = 0, \quad \kappa = 0, \quad A_{\alpha\beta} = \eta_{\alpha\beta} \Phi, \quad P^2 \Phi = m^2 \Phi; \quad (1.12)$$

(ii) a scalar mode, associated to a traceless tensor

$$\lambda = -8m^2, \quad \kappa = 0, \quad A_{\alpha\beta} = \left( P_\alpha P_\beta - \frac{1}{4} \eta_{\alpha\beta} P^2 \right) \Omega, \quad P^2 \Omega = m^2 \Omega; \quad (1.13)$$

(iii) a transverse vector, associated to a traceless tensor

$$\lambda = -6m^2, \quad \kappa = -2m^2, \quad A_{\alpha\beta} = P_\alpha V_\beta + P_\beta V_\alpha, \quad P^\alpha V_\alpha = 0, \quad P^2 V_\alpha = m^2 V_\alpha; \quad (1.14)$$

(iv) a transverse, traceless tensor

$$\lambda = -2m^2, \quad \kappa = -6m^2, \quad A_\alpha{}^\alpha = 0, \quad P^\alpha A_{\alpha\beta} = 0, \quad P^2 A_{\alpha\beta} = m^2 A_{\alpha\beta}. \quad (1.15)$$

e) Check that in all cases the eigenvalues of  $W^2$  satisfy the relation

$$-\frac{\kappa}{m^2} = s(s+1), \quad (1.16)$$

where  $s = 0$  for scalars,  $s = 1$  for vectors and  $s = 2$  for pure symmetric tensors.

## 2 Field equations for anti-symmetric tensor field

Let  $t_{\mu\nu} = -t_{\nu\mu}$  be an anti-symmetric tensor field. Define the operators

$$\theta_{\mu\nu} = \eta_{\mu\nu} - \frac{P_\mu P_\nu}{P^2}, \quad \omega_{\mu\nu} = \frac{P_\mu P_\nu}{P^2}. \quad (2.1)$$

a) Show that one can define two projection operators for  $t_{\mu\nu}$

$$\Pi_{\mu\nu}^{(0)\kappa\lambda} = \frac{1}{2} (\theta_\mu^\kappa \theta_\nu^\lambda - \theta_\mu^\lambda \theta_\nu^\kappa), \quad \Pi_{\mu\nu}^{(1)\kappa\lambda} = \frac{1}{2} (\theta_\mu^\kappa \omega_\nu^\lambda - \theta_\nu^\kappa \omega_\mu^\lambda - \theta_\mu^\lambda \omega_\nu^\kappa + \theta_\nu^\lambda \omega_\mu^\kappa), \quad (2.2)$$

satisfying the properties

$$\Pi^{(A)} \cdot \Pi^{(B)} = \delta^{AB} \Pi^{(A)}, \quad \Pi^{(0)} + \Pi^{(1)} = 1, \quad (2.3)$$

where the unit operator on anti-symmetric tensors is

$$1 \rightarrow \frac{1}{2} (\delta_\mu^\kappa \delta_\nu^\lambda - \delta_\nu^\kappa \delta_\mu^\lambda).$$

b) Consider the field equation

$$\square \Pi_{\mu\nu}^{(0)\kappa\lambda} t_{\kappa\lambda} = m^2 t_{\mu\nu}. \quad (2.4)$$

Check that it is regular (no poles), and that for  $m^2 > 0$  it implies

$$\partial^\lambda t_{\lambda\mu} = 0, \quad \square t_{\mu\nu} = m^2 t_{\mu\nu}, \quad (2.5)$$

*i.e.*, the field is divergence-free and satisfies the Klein-Gordon equation.

c) Show that the field equation (2.4) can be derived from an action

$$S = \int d^4x \left[ -\frac{1}{3!} (\partial_\mu t_{\nu\lambda} + \partial_\nu t_{\lambda\mu} + \partial_\lambda t_{\mu\nu})^2 - \frac{m^2}{2} t_{\mu\nu}^2 \right]. \quad (2.6)$$

d) Check that in the massless case  $m^2 = 0$ , both the action and the field equation are invariant under Abelian gauge transformations

$$t'_{\mu\nu} = t_{\mu\nu} + \partial_\mu \xi_\nu - \partial_\nu \xi_\mu. \quad (2.7)$$

The first term in Eq. (2.6) can be written as  $H_{\mu\nu\lambda}^2$ , with  $H_{\mu\nu\lambda} \equiv \partial_{[\mu} t_{\nu\lambda]}$ . The totally antisymmetric tensor  $H_{\mu\nu\lambda}$  is gauge invariant and can be interpreted as the field strength of  $t_{\mu\nu}$ , thus generalising electrodynamics to a higher rank tensor. The antisymmetric tensor field  $t_{\mu\nu}$  is known as the Kalb-Ramond field and arises naturally in the low energy effective action of the bosonic string, see *e.g.* Ref. [?].

e) Explain how these gauge transformations can be used to obtain the condition that  $t_{\mu\nu}$  is divergence-free, also in the massless case.

### 3 Linearised General Relativity and gravitational waves

#### 3.1 Einstein-Hilbert action

The Einstein form of the action for General Relativity is

$$S = \frac{1}{2\kappa^2} \int d^4x \sqrt{-g} g^{\mu\nu} (\Gamma_{\mu\lambda}^\kappa \Gamma_{\nu\kappa}^\lambda - \Gamma_{\mu\nu}^\lambda \Gamma_{\lambda\kappa}^\kappa). \quad (3.1)$$

The metric connection is

$$\Gamma_{\mu\nu}^\lambda = \frac{1}{2} g^{\lambda\kappa} (\partial_\mu g_{\nu\kappa} + \partial_\nu g_{\mu\kappa} - \partial_\kappa g_{\mu\nu}). \quad (3.2)$$

a) Show that

$$\partial_\lambda g_{\mu\nu} = \Gamma_{\lambda\mu}^\kappa g_{\kappa\nu} + \Gamma_{\lambda\nu}^\kappa g_{\mu\kappa}, \quad (3.3)$$

and that

$$\partial_\mu \sqrt{-g} = \sqrt{-g} \Gamma_{\mu\nu}^\nu. \quad (3.4)$$

b) By partial integration derive the identities

$$\begin{aligned} \int d^4x \sqrt{-g} g^{\mu\nu} \Gamma_{\mu\kappa}^\lambda \Gamma_{\nu\lambda}^\kappa &= \frac{1}{2} \int d^4x \sqrt{-g} g^{\mu\nu} (\partial_\lambda \Gamma_{\mu\nu}^\lambda + \Gamma_{\mu\nu}^\lambda \Gamma_{\lambda\kappa}^\kappa), \\ \int d^4x \sqrt{-g} g^{\mu\nu} \Gamma_{\mu\nu}^\lambda \Gamma_{\lambda\kappa}^\kappa &= \int d^4x \sqrt{-g} g^{\mu\nu} \partial_\mu \Gamma_{\nu\lambda}^\lambda, \end{aligned} \quad (3.5)$$

which hold up to boundary terms.

c) Using these results show that

$$\begin{aligned} S &= \frac{1}{2\kappa^2} \int d^4x \sqrt{-g} g^{\mu\nu} (\partial_\lambda \Gamma_{\mu\nu}^\lambda - \partial_\mu \Gamma_{\nu\lambda}^\lambda - \Gamma_{\mu\kappa}^\lambda \Gamma_{\nu\lambda}^\kappa + \Gamma_{\mu\nu}^\lambda \Gamma_{\lambda\kappa}^\kappa) \\ &= -\frac{1}{2\kappa^2} \int d^4x \sqrt{-g} R. \end{aligned} \quad (3.6)$$

For the last question assume our conventions for the Riemann curvature tensor

$$R_{\mu\nu\kappa}^\lambda \equiv \partial_\mu \Gamma_{\nu\kappa}^\lambda - \partial_\nu \Gamma_{\mu\kappa}^\lambda - \Gamma_{\mu\kappa}^\sigma \Gamma_{\nu\sigma}^\lambda + \Gamma_{\nu\kappa}^\sigma \Gamma_{\mu\sigma}^\lambda.$$

#### 3.2 Linearised equations of motion and gravitational waves

The field equation for the massless spin two field in Minkowski spacetime is

$$\square h_{\mu\nu} - \partial_\mu \partial_\lambda h_\nu^\lambda - \partial_\nu \partial_\lambda h_\mu^\lambda + \partial_\mu \partial_\nu h_\lambda^\lambda - \eta_{\mu\nu} (\square h_\lambda^\lambda - \partial_\kappa \partial_\lambda h^{\kappa\lambda}) = -\kappa T_{\mu\nu}. \quad (3.7)$$

a) Check that the equation is invariant under gauge transformations

$$\delta h_{\mu\nu} = \partial_\mu \xi_\nu + \partial_\nu \xi_\mu. \quad (3.8)$$

b) The Einstein equations can be simplified by switching to different field variables

$$\bar{h}_{\mu\nu} = h_{\mu\nu} - \frac{1}{2} \eta_{\mu\nu} h^\lambda{}_\lambda. \quad (3.9)$$

Show that

$$h_{\mu\nu} = \bar{h}_{\mu\nu} - \frac{1}{2} \eta_{\mu\nu} \bar{h}^\lambda{}_\lambda, \quad (3.10)$$

and rewrite the Einstein equations in terms of  $\bar{h}_{\mu\nu}$ :

$$\square \bar{h}_{\mu\nu} - \partial_\mu \partial_\lambda \bar{h}^\lambda{}_\nu - \partial_\nu \partial_\lambda \bar{h}^\lambda{}_\mu + \eta_{\mu\nu} \partial_\kappa \partial_\lambda \bar{h}^{\kappa\lambda} = -8\pi G T_{\mu\nu}. \quad (3.11)$$

Check the invariance under the modified gauge transformations

$$\bar{h}'_{\mu\nu} = \bar{h}_{\mu\nu} + \partial_\mu \xi_\nu + \partial_\nu \xi_\mu - \eta_{\mu\nu} \partial_\lambda \xi^\lambda. \quad (3.12)$$

c) Define the momentum components  $\varepsilon_{\mu\nu}(k)$  of the redfined spin two field  $\bar{h}_{\mu\nu}$  by

$$\bar{h}_{\mu\nu}(x) = \int \frac{d^4 k}{(2\pi)^2} \varepsilon_{\mu\nu}(k) e^{-ik \cdot x}. \quad (3.13)$$

Prove that the reality of  $\bar{h}_{\mu\nu}$  requires  $\varepsilon_{\mu\nu}^*(k) = \varepsilon_{\mu\nu}(-k)$ , and show that in empty space ( $T_{\mu\nu} = 0$ )

$$k^2 \varepsilon_{\mu\nu} - k_\mu k^\lambda \varepsilon_{\lambda\nu} - k_\nu k^\lambda \varepsilon_{\lambda\mu} + \eta_{\mu\nu} k^\kappa k^\lambda \varepsilon_{\kappa\lambda} = 0, \quad (3.14)$$

and derive the corresponding gauge transformations in momentum space:

$$\varepsilon'_{\mu\nu} = \varepsilon_{\mu\nu} + k_\mu \alpha_\nu + k_\nu \alpha_\mu - \eta_{\mu\nu} k^\lambda \alpha_\lambda, \quad (3.15)$$

with

$$\xi_\mu = i \int \frac{d^4 k}{(2\pi)^2} \alpha_\mu(k) e^{-ik \cdot x}, \quad \alpha_\mu^*(k) = -\alpha_\mu(-k).$$

d) Show that one can find a gauge transformation parameter  $\alpha_\mu$  such that

$$k^\mu \varepsilon'_{\mu\nu} = 0 \quad \text{and} \quad k^2 \varepsilon'_{\mu\nu} = 0. \quad (3.16)$$

This implies that  $\varepsilon'_{\mu\nu}(k) \neq 0$  only on the light cone  $k^2 = 0$ :

$$\varepsilon'_{\mu\nu}(k) = e_{\mu\nu}(\mathbf{k}, \omega_{\mathbf{k}}) \delta(k^2), \quad (3.17)$$

and that the metric perturbation can be expanded as

$$\bar{h}_{\mu\nu}(x) = \int \frac{d^3\mathbf{k}}{8\pi^2\omega_{\mathbf{k}}} \left( e_{\mu\nu}(\mathbf{k}, \omega_{\mathbf{k}}) e^{-i(\mathbf{k}\cdot\mathbf{r}-\omega_{\mathbf{k}}t)} + e_{\mu\nu}^*(\mathbf{k}, \omega_{\mathbf{k}}) e^{i(\mathbf{k}\cdot\mathbf{r}-\omega_{\mathbf{k}}t)} \right), \quad (3.18)$$

with the convention  $\omega_{\mathbf{k}} = \sqrt{\mathbf{k}^2}$ .

e) Check, that the momentum amplitude  $e_{\mu\nu}(\mathbf{k})$  satisfies

$$k_i e_{i\mu} = \omega_{\mathbf{k}} e_{0\mu}, \quad (3.19)$$

and this condition is respected by gauge transformations on the light cone:

$$\alpha_\mu = a_\mu(\mathbf{k}, \omega_{\mathbf{k}}) \delta(k^2),$$

such that

$$\begin{aligned} e'_{00} &= e_{00} + \omega_{\mathbf{k}} a_0 + \mathbf{k} \cdot \mathbf{a}, \\ e'_{i0} &= e_{i0} + k_i a_0 + \omega_{\mathbf{k}} a_i, \\ e'_{ij} &= e_{ij} + k_i a_j + k_j a_i - \delta_{ij} (\mathbf{k} \cdot \mathbf{a} - \omega_{\mathbf{k}} a_0). \end{aligned} \quad (3.20)$$

Find  $(a_0, \mathbf{a})$  such that

$$e'_{00} = e'_{i0} = \sum_{k=1}^3 e'_{kk} = 0. \quad (3.21)$$

*Answer:*

$$a_0 = -\frac{1}{4\omega_{\mathbf{k}}} \left( e_{00} + \sum_k e_{kk} \right), \quad a_i = -\frac{1}{\omega_{\mathbf{k}}} e_{i0} + \frac{k_i}{4\omega_{\mathbf{k}}^2} \left( e_{00} + \sum_k e_{kk} \right). \quad (3.22)$$

f) Explain that there are only 2 polarisation modes for a perturbation with wave vector  $\mathbf{k}$ , and that these can be taken to be space-like, transverse and traceless:

$$e_{00} = e_{i0} = 0, \quad \sum_i k_i e_{ij} = 0, \quad \sum_i e_{ii} = 0. \quad (3.23)$$

In particular explain that for a perturbation mode moving in the  $z$ -direction one can take

$$e_{\mu\nu}(k_z, \omega_{\mathbf{k}}) = A_+(k_z) e_{\mu\nu}^+ + A_\times(k_z) e_{\mu\nu}^\times, \quad (3.24)$$

with

$$e_{\mu\nu}^+ = \begin{pmatrix} 0 & 0 & 0 & 0 \\ 0 & 1 & 0 & 0 \\ 0 & 0 & -1 & 0 \\ 0 & 0 & 0 & 0 \end{pmatrix}, \quad e_{\mu\nu}^\times = \begin{pmatrix} 0 & 0 & 0 & 0 \\ 0 & 0 & 1 & 0 \\ 0 & 1 & 0 & 0 \\ 0 & 0 & 0 & 0 \end{pmatrix}. \quad (3.25)$$

- g)* Prove, that these gauge transformations turn the solutions for the metric perturbations  $\bar{h}_{\mu\nu}$  into a solution of the linearised Einstein equations with the properties

$$\bar{h}_{00} = \bar{h}_{i0} = 0, \quad \sum_i \bar{h}_{ii} = 0, \quad \sum_i \partial_i \bar{h}_{ij} = 0, \quad \square \bar{h}_{ij} = 0. \quad (3.26)$$
